# Supplementary material for: Attosecond tracking of light absorption and refraction in fullerenes
Source: arXiv:1206.7061 source file (2012-06-29)
Supplement: Supplementary file 1 [file supp_mat.pdf]

# Supplemental Material: Attosecond tracking of light absorption and refraction in fullerenes

A.S. Moskalenko, Y. Pavlyukh, and J. Berakdar

## I. SPHERICAL MOLECULES

Recently [1, 2] we devised a scheme to distill the main angular momentum components of the valence electron wave functions of quasi-spherical molecules. In short, we found that the average radial distance is peaked at the value which we call the "radius" $r_0$ of the

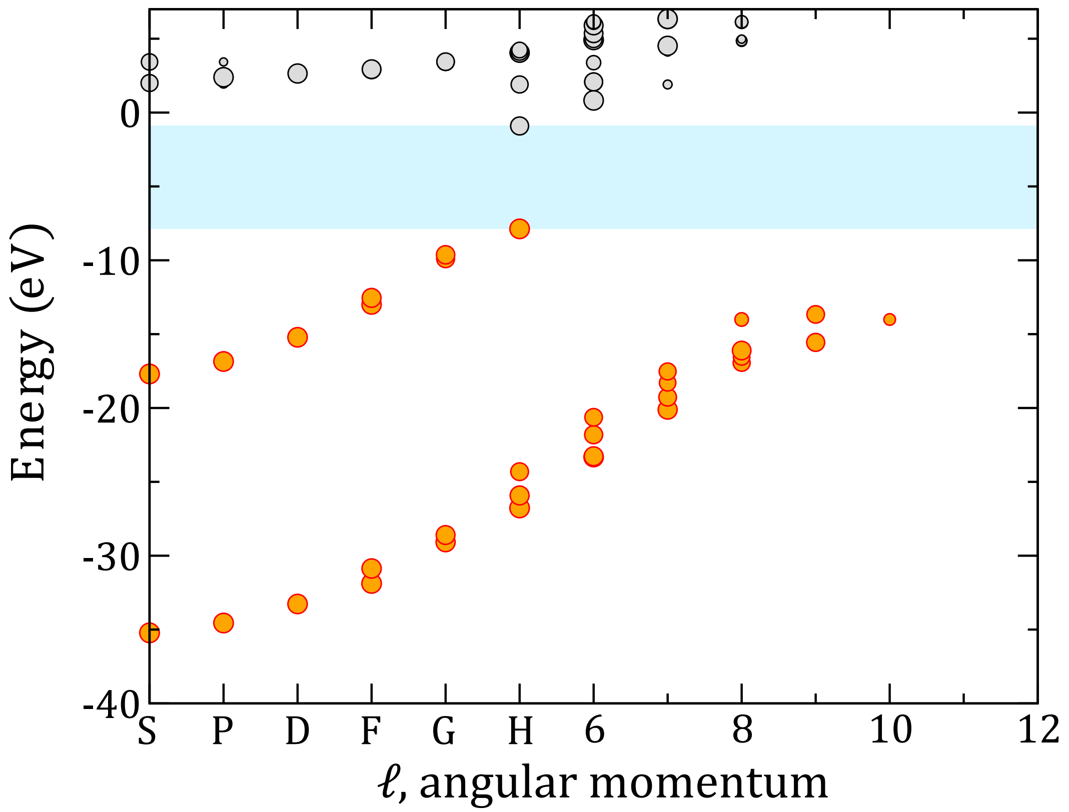


FIG. 1. The valence single-particle energy spectrum $\varepsilon_{n\ell}$ vs. the orbital angular momentum of electrons in the $C_{60}$ molecule is dominated by two radial subbands $\varepsilon_{1\ell}$ and $\varepsilon_{2\ell}$ each dispersing with the angular momentum $\ell \approx r_0 p/\hbar$. Here $r_0$ is the average radius of $C_{60}$ and $p$ can be interpreted as the momentum [1, 2]. The circles (full for occupied and empty circles for unoccupied) show the dominant contributions to the energy spectrum vs. the electron orbital angular momentum, as obtained from *ab-initio* calculations. The gap is marked by the shaded stripe.

molecule. For this distance we expand the wave function $\Psi_\epsilon(\vec{r})$, as determined *ab-initio*, in terms of spherical harmonics with coefficients $c_{\ell m}$. The circles in Fig. 1 show the dominant contributions $\sum_m |c_{\ell m}|^2$ to this expansion in dependence on $\ell$ (their relative size marks their relative weight). Since for a given energy one circle in Fig. 1 is dominant, i.e. one $\ell$, this $\ell$ can be considered as a good quantum number. For the large angular momenta $\ell$ we may interpret the spectrum in Fig. 1 as the band structure, for which we can introduce $p \approx \ell/r_0$ as the averaged momentum. For each circle in Fig. 1 we can thus write the single particle wave function as $\phi_\alpha = R_n(r)Y_{lm}(\Omega)$, where $R_n(r)$ is a radial function with $n-1$ nodes. These states are taken as a basis for expressing the components of the density matrix. Note, the same procedure applies to a series of molecules [1, 2].

---


[1] Y. Pavlyukh and J. Berakdar, Chem. Phys. Lett. **468**, 313 (2009).

[2] Y. Pavlyukh and J. Berakdar, Phys. Rev. A **81**, 042515 (2010).
